# Supplementary material for: FAT: Training Neural Networks for Reliable Inference Under Hardware Faults
Source: arXiv:2011.05873 source file (2020-11-11)
Supplement: Supplementary file 1 [file appendix.tex]

\clearpage
\newpage
\appendix

\input{images/FAT_CNVW1A1.tex}
\input{images/FAT_CNVW2A2.tex}
\input{images/XFAT_CNVW1A2.tex}
\input{images/XFAT_CNVW2A2.tex}
\input{images/XFAT_CNVW1A1_GTSRB.tex}
\input{images/XFAT_CNVW1A1_SVHN.tex}
\input{images/DROPOUT2D_CNVW1A2.tex}
\input{images/DROPOUT2D_CNVW2A2.tex}
